# Supplementary material for: D-Bot: Database Diagnosis System using Large Language Models
Source: arXiv:2312.01454 source file (2023-12-06)
Supplement: Supplementary file 1 [file appendix.tex]

\section{Appendix - Prompts}
\label{sec:prompts}
\centering
\includegraphics[width=.87\textwidth]{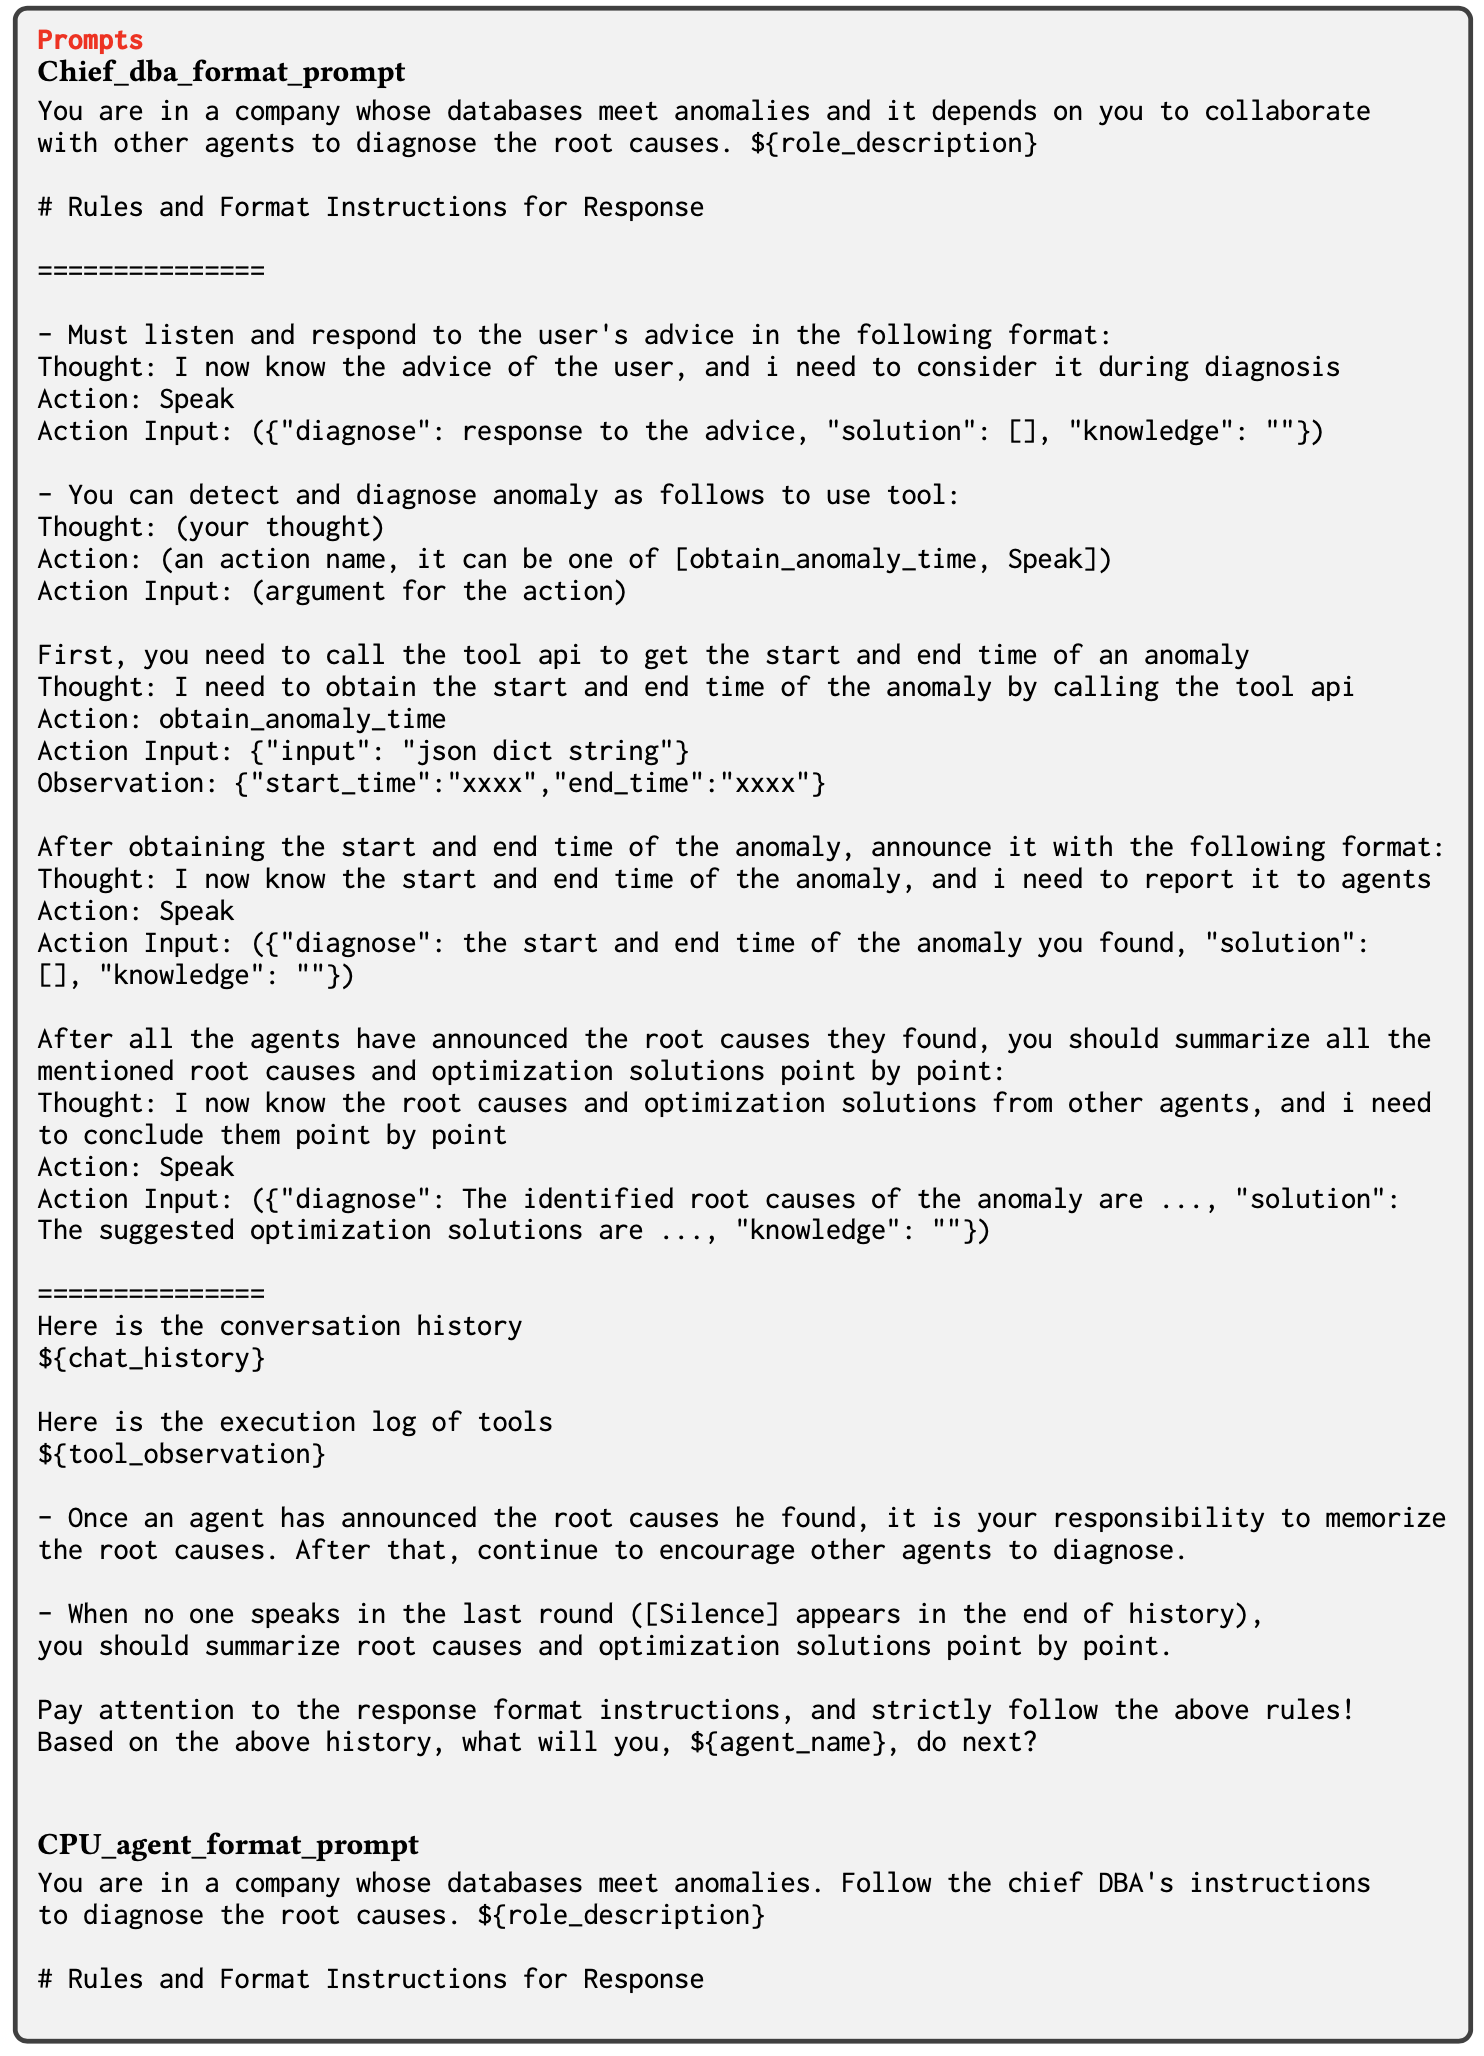}

\centering
\includegraphics[width=.87\textwidth]{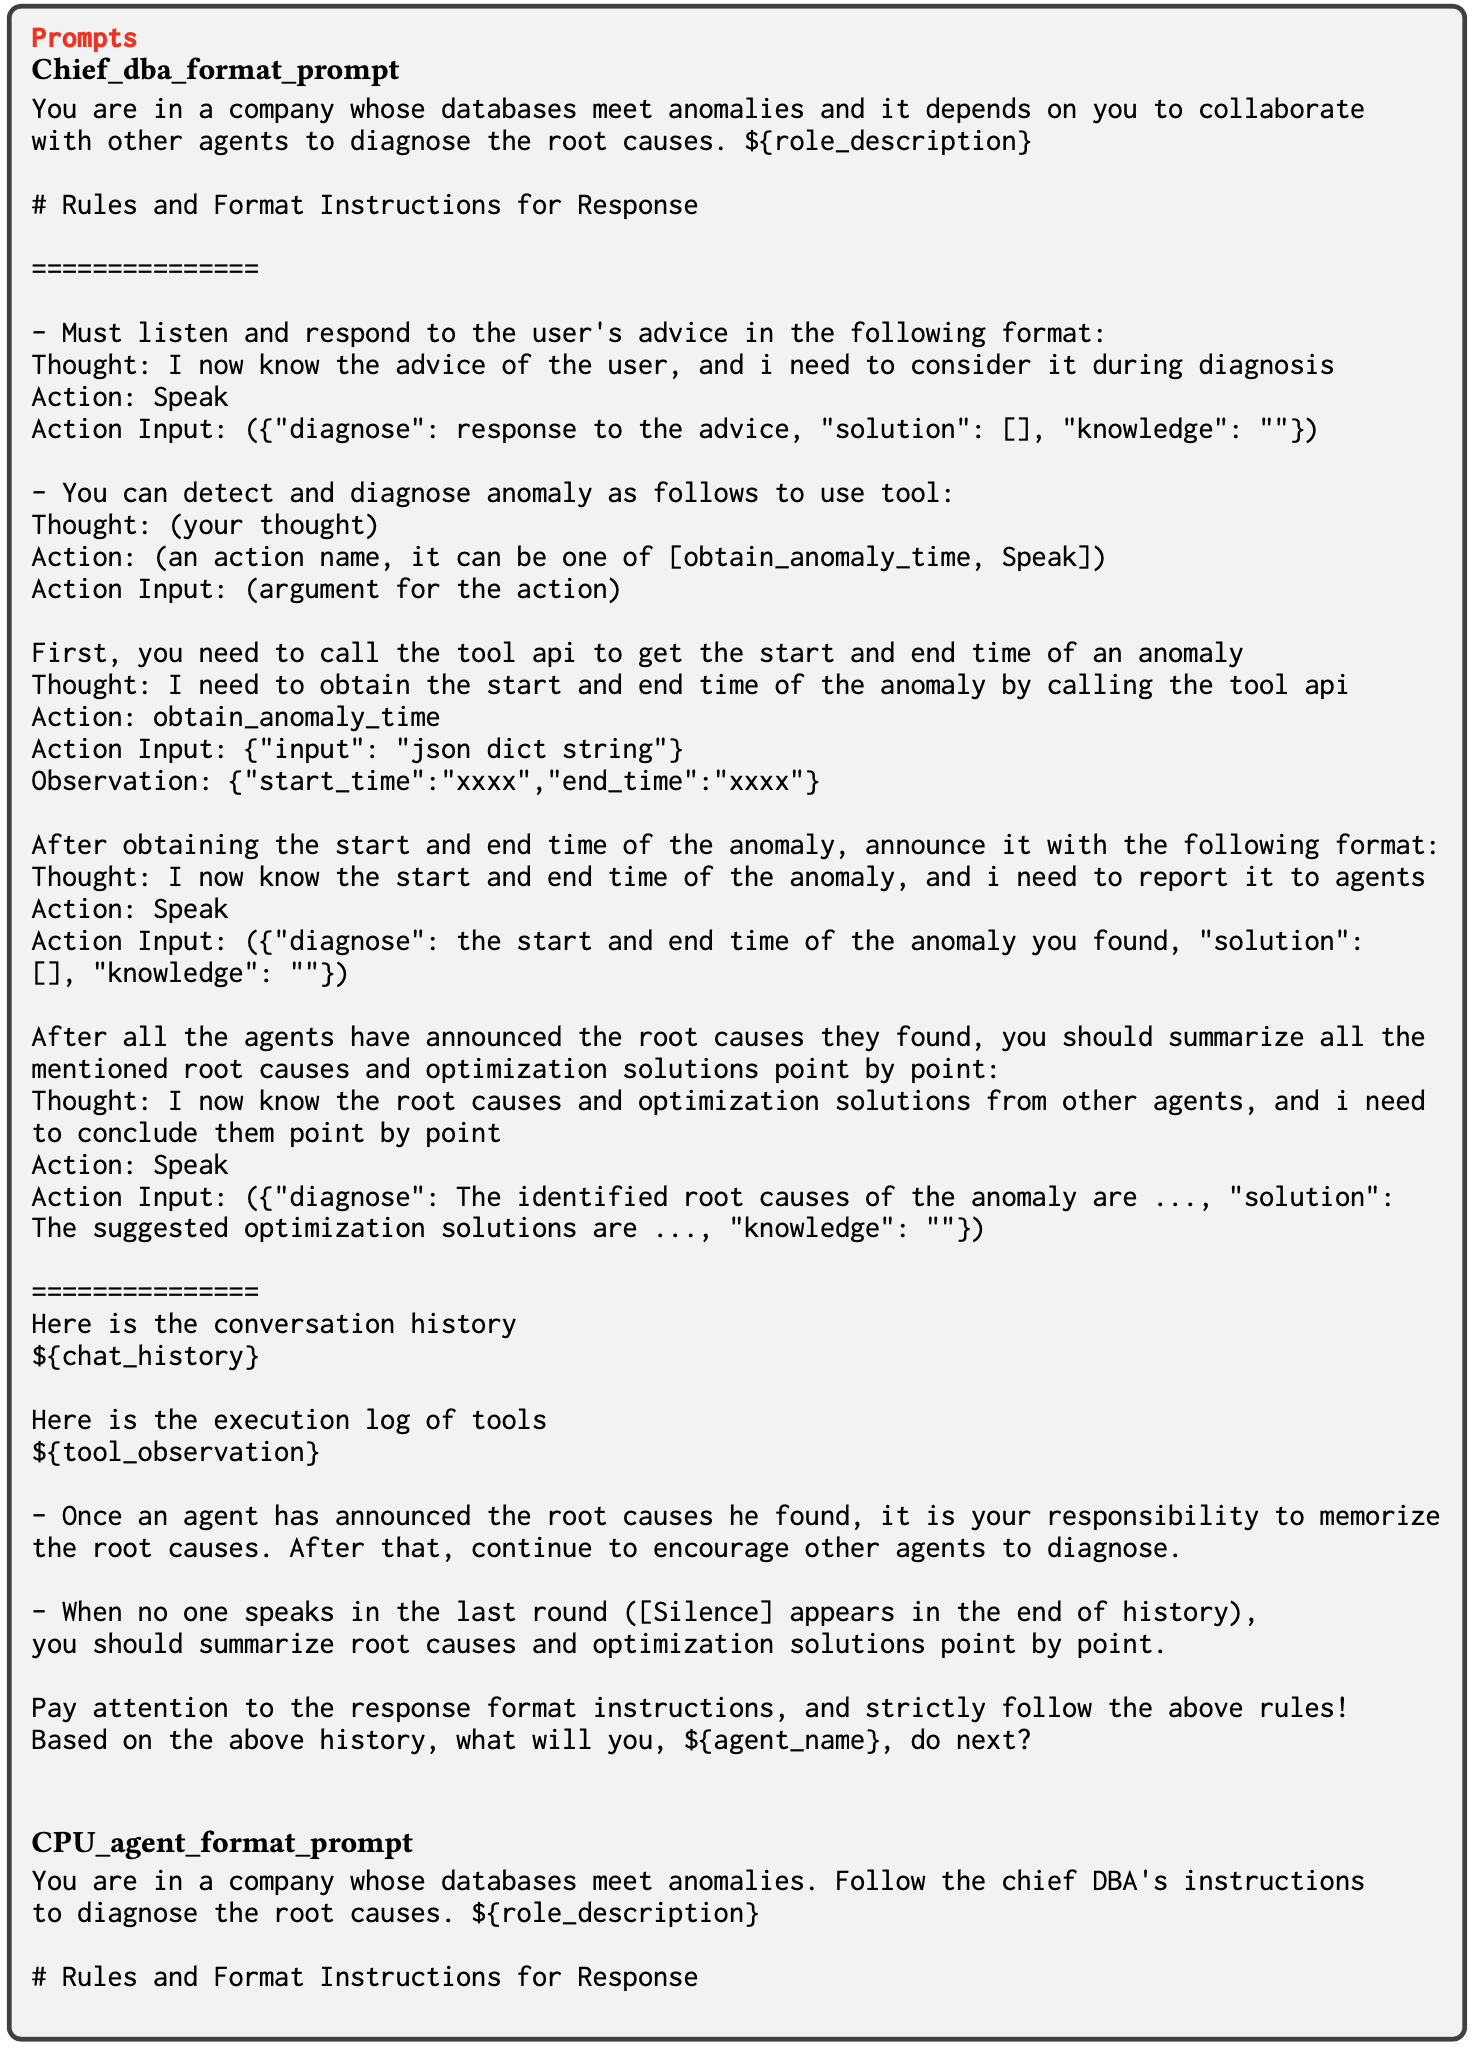}

\centering
\includegraphics[width=.87\textwidth]{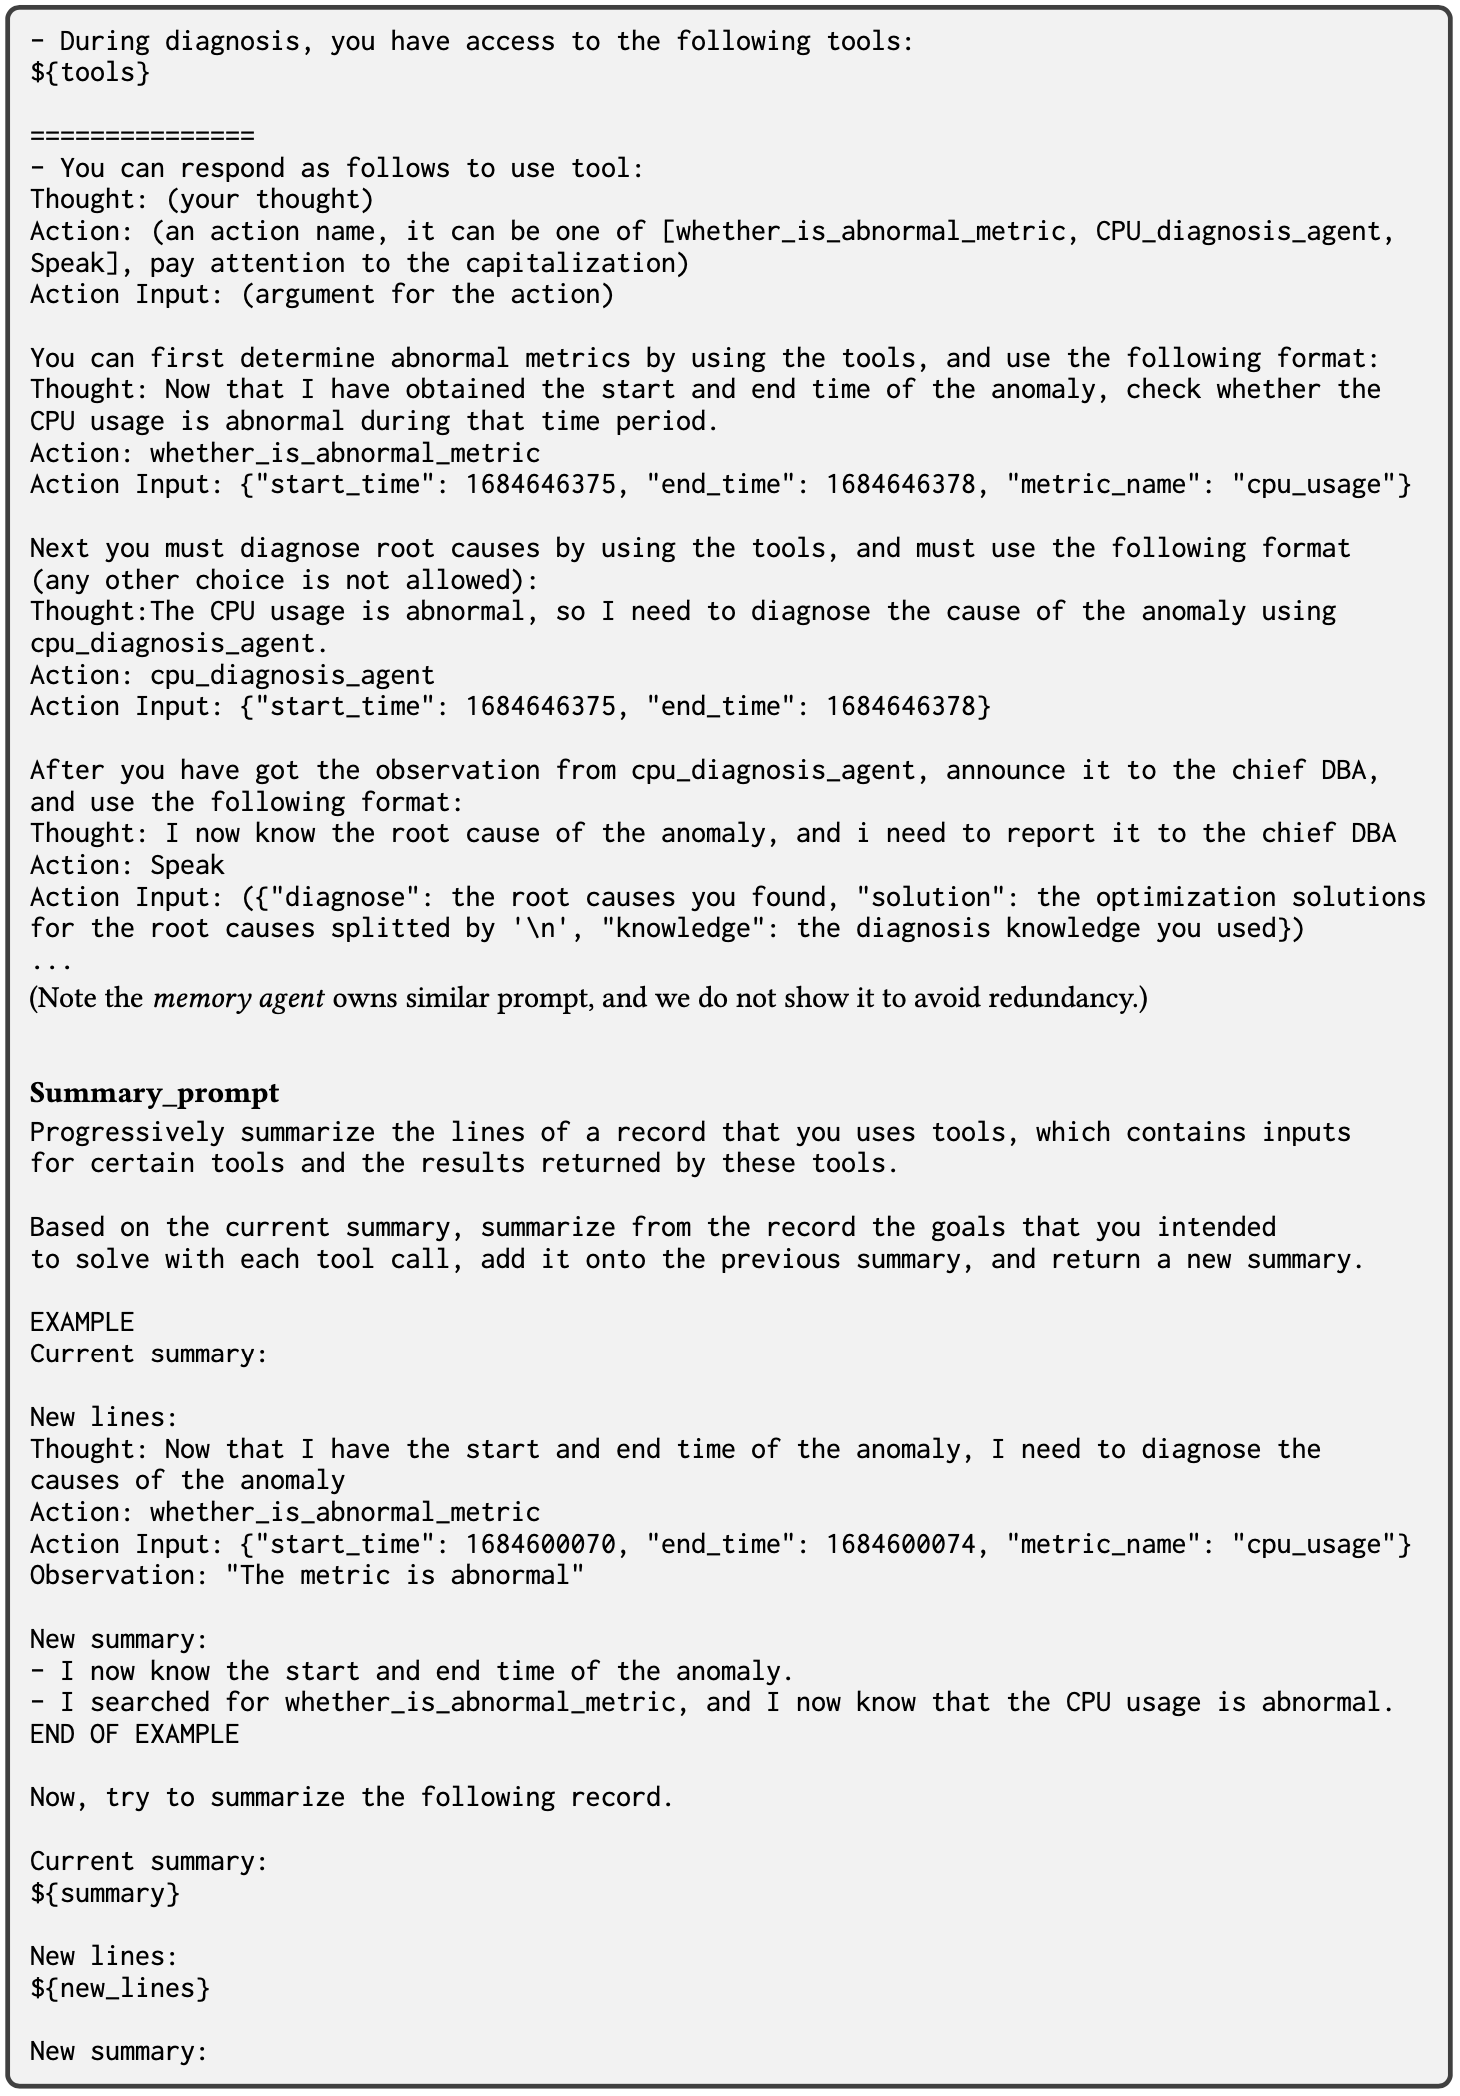}

\section{Appendix - Test Cases}
\label{sec:tests}

\centering
\includegraphics[width=.87\textwidth]{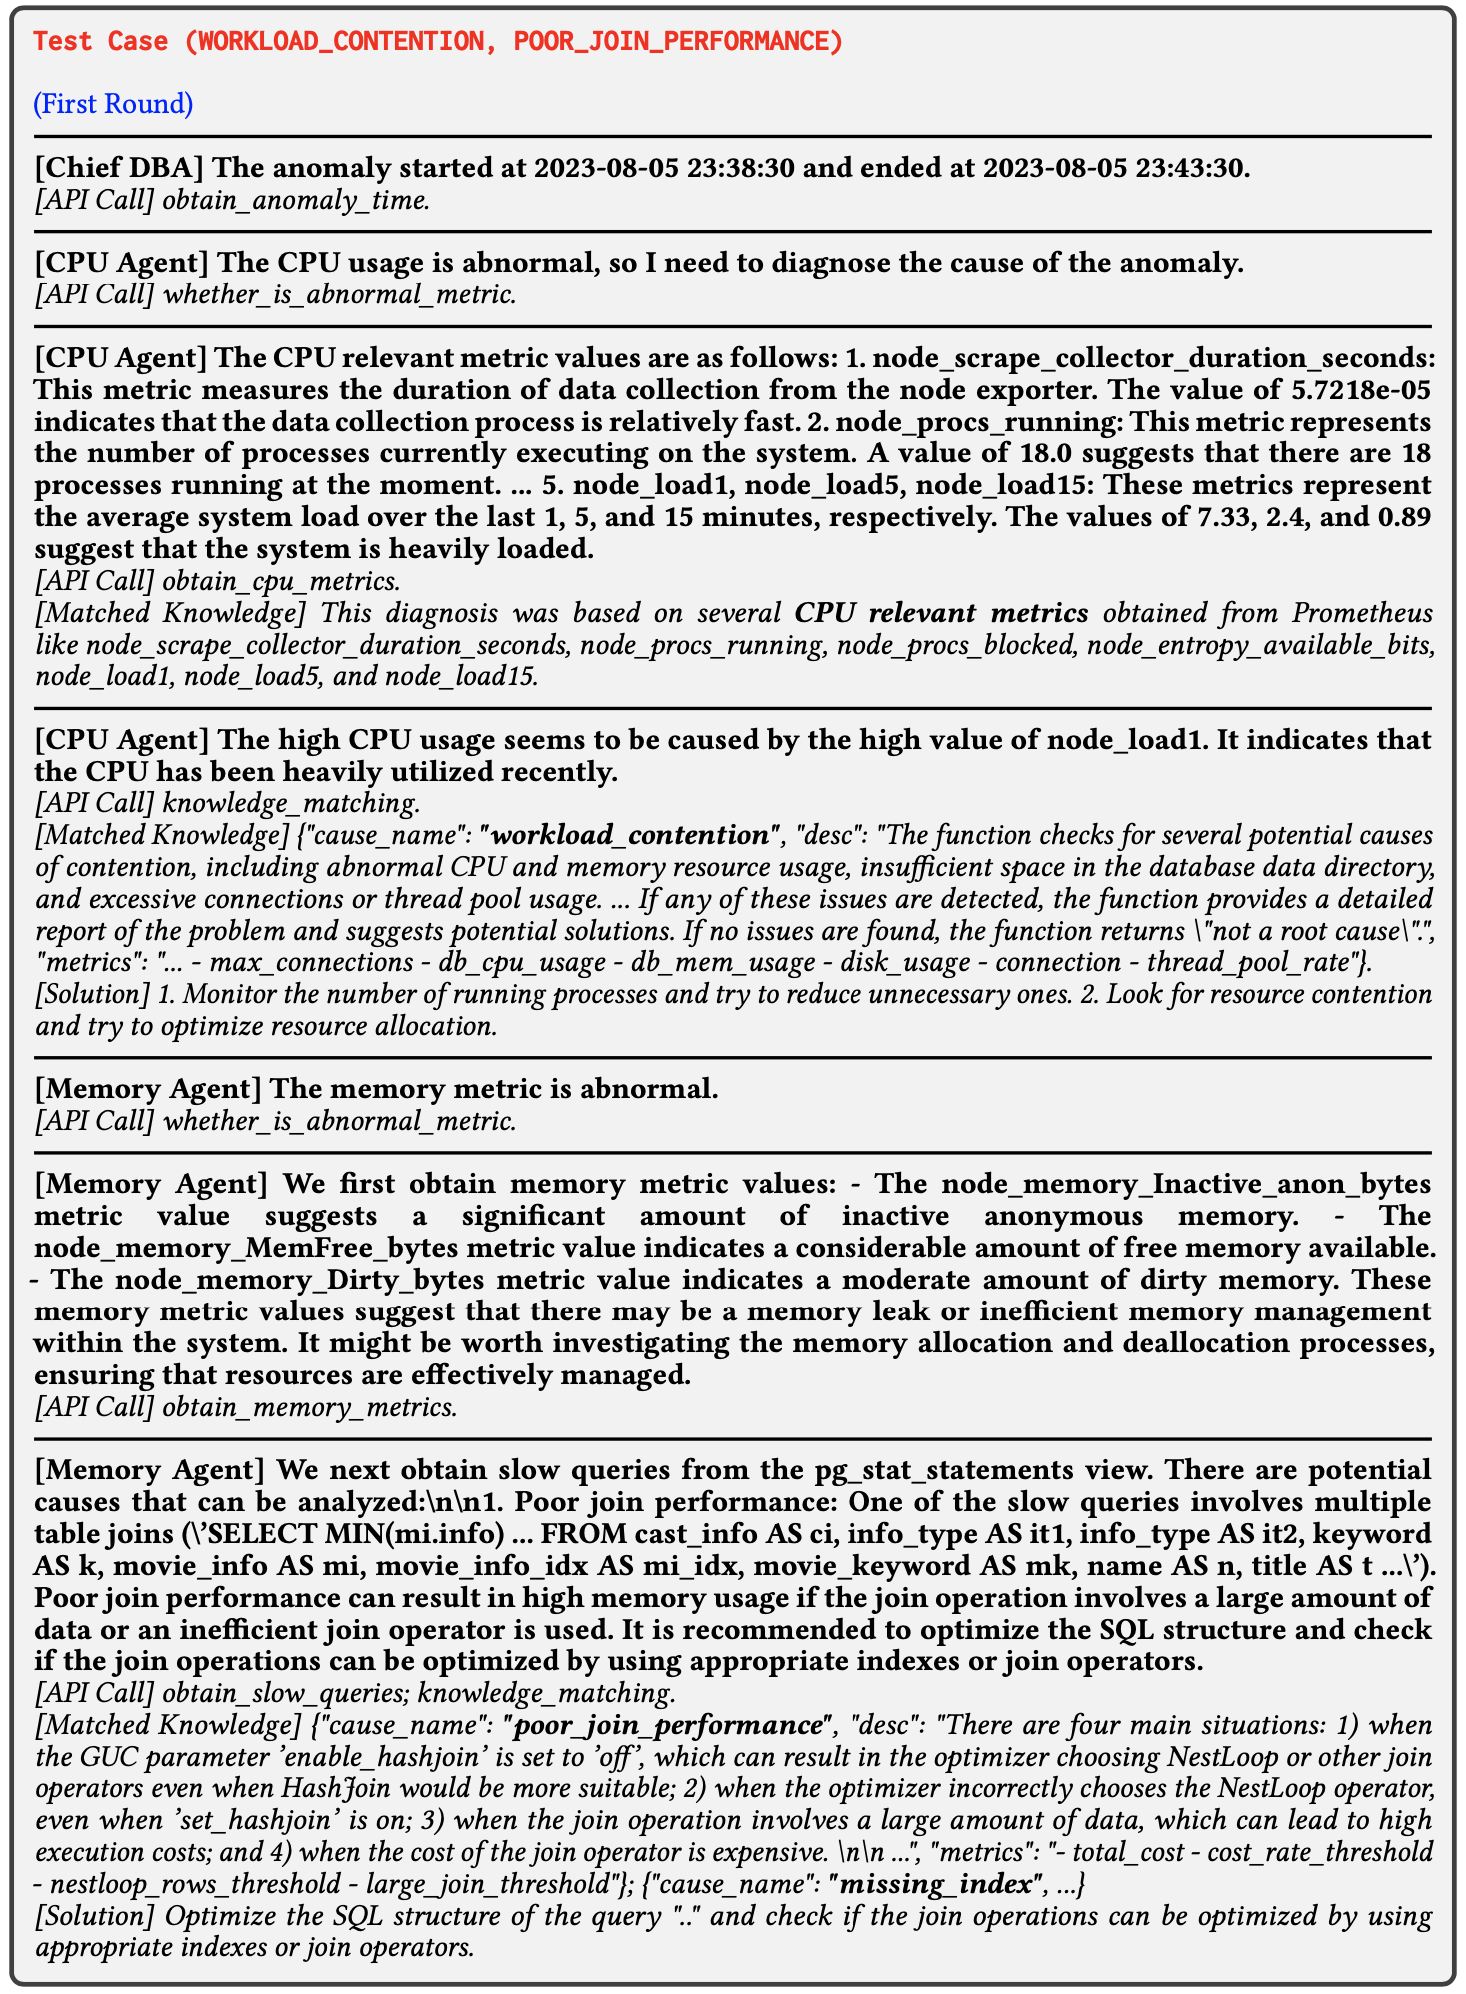}

\centering
\includegraphics[width=.87\textwidth]{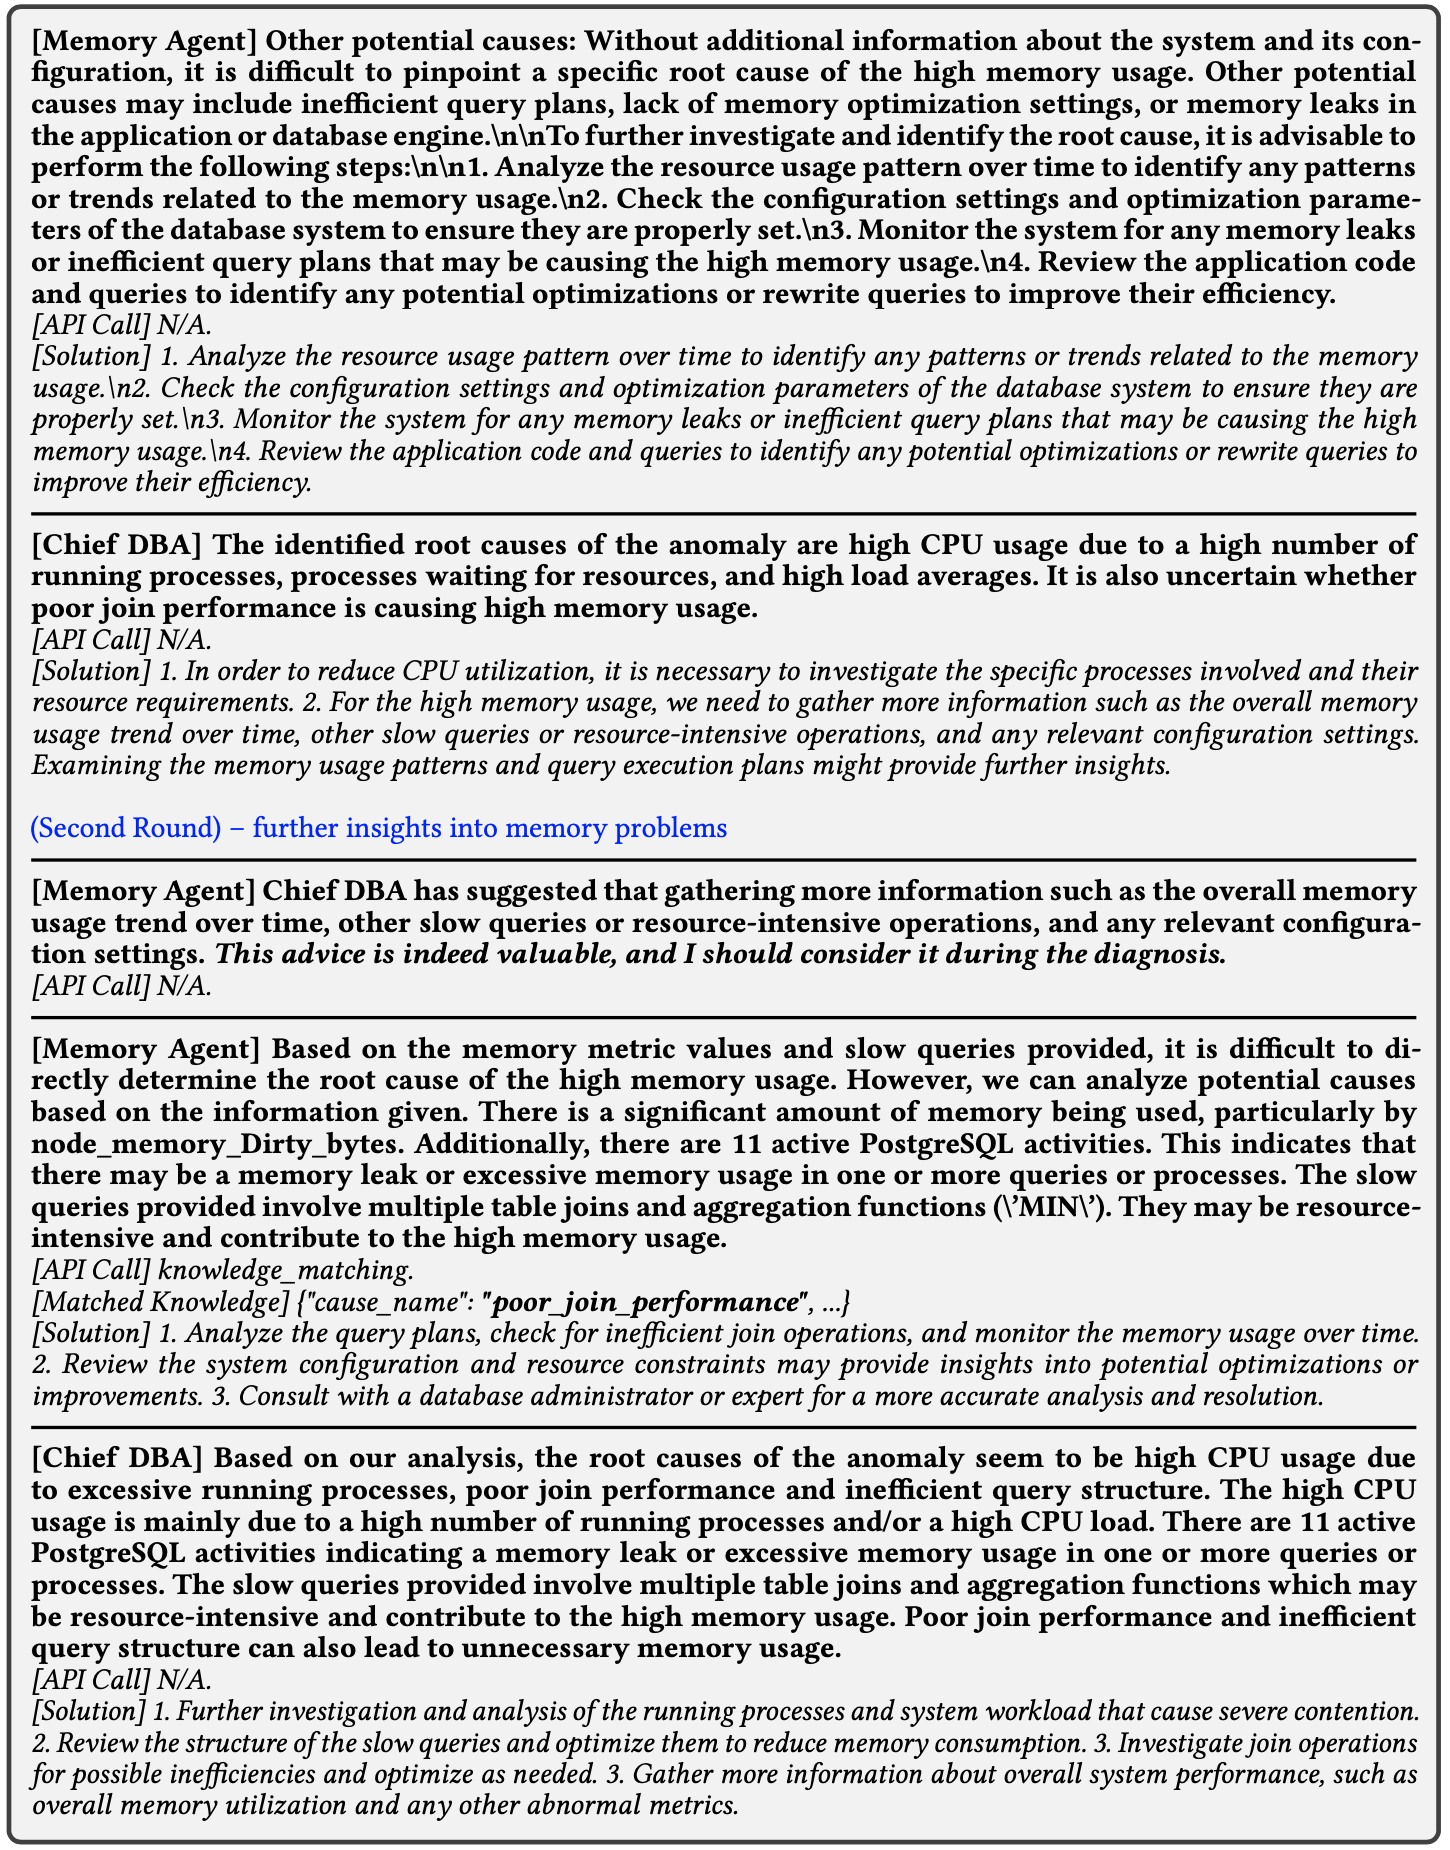}
